# Supplementary material for: Understanding step selection analysis through numerical integration
Source: arXiv:2308.15678 ancillary file (2023-08-30)
Supplement: Supplementary file 1 [file appendices.pdf]

# Appendices for "Understanding step selection analysis through numerical integration''

Théo Michelot, Natasha Klappstein, Jonathan Potts, John Fieberg

## Contents

**A Including the observed location as an integration point** **2**

**B Simulated covariate** **3**

**C Implementing step selection analysis** **4**

C.1 Functions . . . 4

C.2 Example analysis . . . 9

C.3 Examples of sampling distributions . . . 12

**D Implementation of different movement distributions** **16**

D.1 Example: including step length as a covariate . . . 16

D.2 Mathematical justification . . . 19

D.3 From $f_r$ to $f_{x,y}$ . . . 21

D.4 From $f_{x,y}$ to $f_r$ . . . 22

**References** **23**

# A Including the observed location as an integration point

When numerical integration is directly applied to the step selection function model (Equation 1 in the main text), the integral is approximated by a sum where the integrand is evaluated over a set of random or deterministic integration points. We made a slight modification and also included the observed step as an additional integration point, so that the formulas that we present exactly match those derived from discrete-choice models in the literature. Another argument in favour of including the observation is that we have found it to greatly help with parameter estimation in many applications. This is likely because the observed location will usually fall in an area where the SSF is high, and so it is a valuable integration point. In this appendix, we present some simulation results to illustrate the effect of including the observed location as an integration point.

We followed a simulation procedure very similar to that described in Section 3.1 of the main text, but we fitted each model twice: once with the observed location included in the sum, and once without it. We considered two model fitting methods, one based on uniform Monte Carlo sampling, and one based on importance sampling with gamma-distributed distances and von Mises-distributed turning angles. Figure S1 shows the results of the simulation, comparing estimation bias for the two estimation methods with or without including the observed location as an integration point. Including the observation clearly decreases bias, particularly in the uniform sampling scheme. In fact, it seems that estimation based on uniform Monte Carlo sampling systematically fails for relatively small numbers of random points, when the observation is excluded from the approximation.

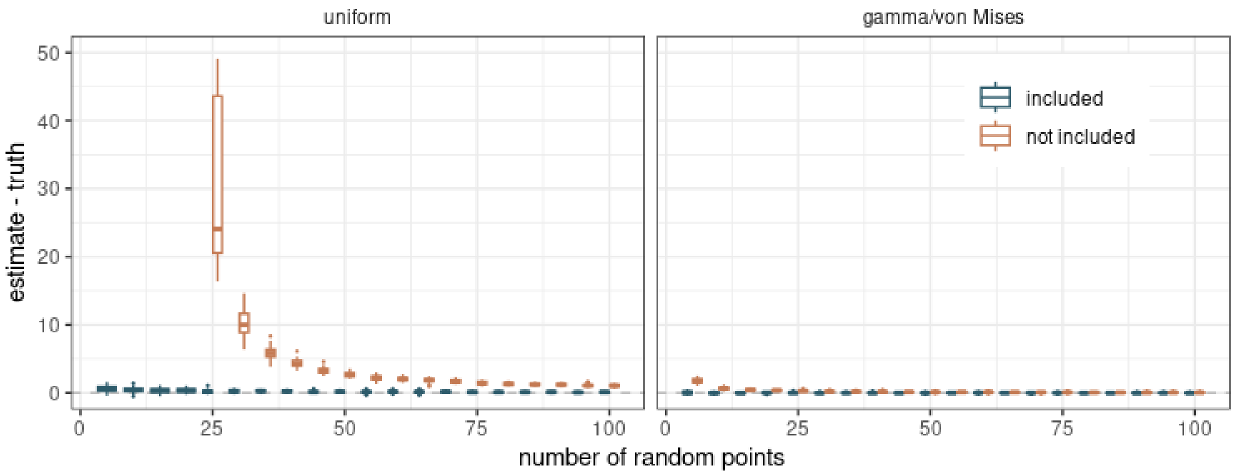


***Figure S1:*** *Results of simulation comparing estimation performance with (blue) and without (orange) the observed location included as an integration point. Each box represents 50 bias estimates. For the uniform sampling scenario, some boxes are missing because optimisation failed.*

# B Simulated covariate

In Section 3.1 of the main text, we created a covariate to use in a simulation study of different SSF fitting techniques. We generated the covariate over a raster grid by first sampling uniform values in each grid cell, and then applying a moving average over a circular window to obtain realistic spatial autocorrelation. Figure S2 shows a plot of the simulated covariate over the study region, overlaid with the simulated trajectory.

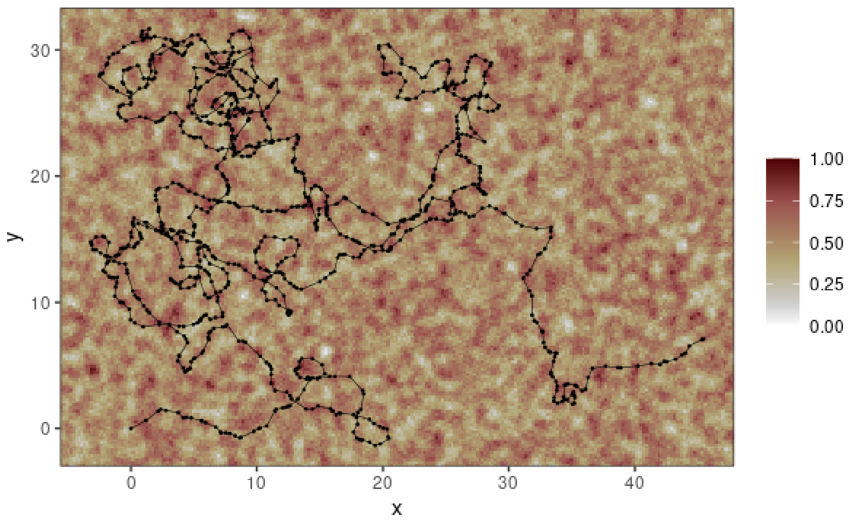


***Figure S2:*** *Artificial raster layer used as spatial covarite in simulation study, and simulated track.*

# C Implementing step selection analysis

A general inferential method for step selection analysis is to implement the likelihood function and optimise it directly for parameter estimation. For experienced users, this approach can greatly increase the flexibility in terms of modelling and method of inference, compared to conditional logistic regression. In this document, we provide documented R code that can be used as a template to write custom step selection analyses. It implements the importance sampling approach described in the paper, which includes other approaches as special cases.

We focus on the case where both the habitat selection function $w$ and the movement kernel $\phi$ take an exponential form, i.e., $w(\boldsymbol{x}_t, \boldsymbol{x}_{t+1}) = \exp(c_m(\boldsymbol{x}_t, \boldsymbol{x}_{t+1})\boldsymbol{\beta}_m^\intercal)$ and $\phi(\boldsymbol{x}_{t+1} \mid \boldsymbol{x}_{1:t}) = \exp(c_h(\boldsymbol{x}_t, \boldsymbol{x}_{t+1})\boldsymbol{\beta}_h^\intercal)$, where $c_m$ (resp. $c_h$) returns a vector of movement variables (resp. habitat variables) and $\boldsymbol{\beta}_m$ (resp. $\boldsymbol{\beta}_h$) is the vector of associated selection parameters. The SSF can then be factorised, yielding the model presented below where $c(\boldsymbol{x}_t, \boldsymbol{x}_{t+1})$ contains both movement and habitat variables, and $\boldsymbol{\beta}$ contains both movement and habitat selection coefficients. For a more detailed derivation, see Klappstein, Thomas, and Michelot (2023).

## C.1 Functions

The R code that we provide is based on three functions:

- `nllk_ssf()` computes the negative log-likelihood;
- `ssf()` uses the optimiser `optim()` to find the maximum likelihood estimates;
- `add_random()` generates random points for the numerical integration. Alternatively, `amt::random_steps()` can be used.

### C.1.1 Negative log-likelihood

Based on the assumption that steps are independent, the likelihood of a track is the product of the step likelihoods,

$$L = \prod_{t=1}^{n-1} \frac{\exp\left[c(\boldsymbol{x}_t, \boldsymbol{x}_{t+1})\boldsymbol{\beta}^\intercal\right]}{\sum_{k=0}^{K} \frac{\exp[c(\boldsymbol{x}_t, \boldsymbol{z}_{tk})\boldsymbol{\beta}^\intercal]}{h(\boldsymbol{x}_t, \boldsymbol{z}_{tk})}}$$

It is common statistical practice to consider the log-likelihood rather than the likelihood, to avoid numerical problems such as underflow and overflow. Defining the log-likelihood as $\ell = \log(L)$, we find

$$\begin{aligned}
\ell &= \sum_{t=1}^{n-1} \log \left( \frac{\exp\left[c(\boldsymbol{x}_t, \boldsymbol{x}_{t+1})\boldsymbol{\beta}^\intercal\right]}{\sum_{k=0}^{K} \frac{\exp[c(\boldsymbol{x}_t, \boldsymbol{z}_{tk})\boldsymbol{\beta}^\intercal]}{h(\boldsymbol{x}_t, \boldsymbol{z}_{tk})}} \right) \\
&= \sum_{t=1}^{n-1} \left\{ c(\boldsymbol{x}_t, \boldsymbol{x}_{t+1})\boldsymbol{\beta}^\intercal - \log \sum_{k=0}^{K} \frac{\exp\left[c(\boldsymbol{x}_t, \boldsymbol{z}_{tk})\boldsymbol{\beta}^\intercal\right]}{h(\boldsymbol{x}_t, \boldsymbol{z}_{tk})} \right\}
\end{aligned}$$

To implement this formula in R, we loop over the strata ($t$ variable in the equation), and compute the likelihood for each stratum as shown above. Note that we return the negative log-likelihood ($-\ell$) because the optimisation is carried out using `nlm()`, which is a *minimiser*. That is, we seek the parameter values that minimise the negative log-likelihood, which coincide with the maximum likelihood estimates.

```
#' Negative log-likelihood
#'
#' Arguments:
#' par          Vector of SSF parameters
#' mod_mat      Model matrix
#' stratum_ind  Vector of indices at which strata start
#' h            Vector of importance sampling weights
#'
#' Return: Single number
nllk_ssf <- function(par, mod_mat, stratum_ind, h) {
    # Compute log-SSF (linear predictor)
    log_ssf <- mod_mat %*% par
    # Set SSF to zero if NA
    log_ssf[is.na(log_ssf)] <- -Inf
    # Compute log-SSF scaled by importance function
    log_ssf_scaled <- log_ssf - log(h)

    # Loop over strata
    llk_all <- rep(0, length(stratum_ind) - 1)
    for(i in 1:(length(stratum_ind) - 1)) {
        # Index of observation for this stratum
        ind_obs <- stratum_ind[i]
        # Indices of random points for this stratum
        ind_random <- stratum_ind[i]:(stratum_ind[i+1] - 1)

        # Scaling constant (to avoid numerical issues - cancels out)
        c <- max(log_ssf_scaled[ind_random])
        if(is.finite(c)) {
            # Save likelihood for this stratum
            llk_all[i] <- log_ssf[ind_obs] -
                (c + log(sum(exp(log_ssf_scaled[ind_random] - c))))
        }
    }
```

```
    # Return negative log-likelihood
    return(- sum(llk_all))
}
```

The first line of `nllk_ssf()` evaluates the log of the SSF at all the points as a product of the model matrix (which includes habitat as well as movement variables) and the vector of selection parameters. This is because we have assumed that the SSF is in exponential form, but the movement component of `log_ssf` could instead be computed using another function (e.g., `dweibull()` for a Weibull step length distribution).

### C.1.2 Model fitting

Any numerical optimiser can be used on `nllk_ssf()` to find the maximum likelihood estimates of the SSF parameters; some popular choices include `nlm()`, `nlminb()`, and `optim()`. Here, we use `nlm()`. Before we can optimise the negative log-likelihood, we need to prepare the arguments to pass to `nllk_ssf()`.

1. We create a model (design) matrix from the formula and data frame (passed as the argument `mat`).
2. We identify the indices at which a new stratum starts, which is used to loop over strata in the likelihood (passed as the argument `stratum_ind`).
3. We evaluate the importance sampling weights, which are then passed to the likelihood function as the argument `h`.

The output of `nlm()` includes the minimum value of the negative log-likelihood, as well as the vector of maximum likelihood estimates of the model parameters, and a convergence code. (See `?nlm` for more detail.)

```
#' Fit step selection function
#'
#' Arguments:
#' formula      SSF formula
#' data         Data frame with named columns "sl_" (step length), "ta_"
#'              (turning angle), "case_" (0/1 to identify observed and random
#'              locations), "step_id_" (stratum identifier), and each covariate
#'              in the formula
#' par0         Vector of starting values for the SSF parameters
#' dsamp        Probability density function of the importance distribution
#' ...          Named arguments for dsamp()
#'
#' Return: output of nlm()
```

```r
ssf <- function(formula, data, par0, dsamp, ...) {
    # Model matrix (passing NAs and removing intercept)
    mat <- model.matrix.lm(update.formula(formula, "~ . - 1"),
                           data = data, na.action = "na.pass")

    # Find indices of strata
    strat_ind <- c(1, cumsum(rle(data$step_id_)$lengths) + 1)

    # Importance sampling weights
    h <- dsamp(data$sl_, data$ta_, ...)

    # Optimise likelihood
    mod <- nlm(f = nllk_ssf, p = par0, mod_mat = mat,
               stratum_ind = strat_ind, h = h)

    return(mod)
}
```

### C.1.3 Random locations

We also provide a general function to generate random locations based on a user-defined importance function. The random generator for the importance function, passed as the argument `rsamp` below, must return a list with elements `sl_` (step lengths) and `ta_` (turning angles), for consistency with amt syntax. Alternatively, users familiar with the amt package can use the function `amt::random_steps()`, and we present both workflows in an example in the next section.

```r
#' Generate random points
#'
#' Arguments:
#' data         Data frame with named columns 'x_' and 'y_'
#' n_random     Number of random locations to add for each step
#' rsamp        Random number generator of the importance function, returning
#'              a list with named elements 'sl_' (step lengths) and 'ta_'
#'              (turning angles)
#' ...          Named arguments for rsamp()
#'
#' Return: a data frame with all observed and random steps
add_random <- function(data, n_random, rsamp, ...) {
    # Matrix of locations
    xy <- as.matrix(data[, c("x_", "y_")])
```

```r
    n_obs <- nrow(xy)

    # Get a few movement metrics
    steps <- sqrt(rowSums((xy[-1,] - xy[-n_obs,])^2))
    bears <- atan2(diff(xy[,2]), diff(xy[,1]))
    angles <- diff(bears)
    # Make sure angles are in (-pi, pi]
    angles <- ifelse(angles < -pi, angles %% pi, angles)
    angles <- ifelse(angles > pi, angles %% pi - pi, angles)

    # Loop over observed steps
    data_list <- lapply(3:n_obs, function(i) {
        # Simulate step lengths and turning angles for random steps
        sim_var <- rsamp(n_random, ...)
        sim_step <- sim_var$sl_
        sim_angle <- sim_var$ta_
        # Make sure angles are in (-pi, pi]
        sim_angle <- ifelse(sim_angle < -pi, sim_angle %% pi, sim_angle)
        sim_angle <- ifelse(sim_angle > pi, sim_angle %% pi - pi, sim_angle)
        # Derive coordinates of random points
        sim_bear <- bears[i-2] + sim_angle
        pts <- rep(xy[i-1,], each = length(sim_step)) +
            sim_step * cbind(cos(sim_bear), sin(sim_bear))

        # Output data frame for this stratum
        data.frame(x_ = c(xy[i,1], pts[,1]),
                   y_ = c(xy[i,2], pts[,2]),
                   sl_ = c(steps[i-1], sim_step),
                   ta_ = c(angles[i-2], sim_angle),
                   step_id_ = i,
                   case_ = c(1, rep(0, nrow(pts))))
    })

    # Combine data frames for all strata
    data_all <- do.call(rbind, data_list)
    return(data_all)
}
```

### C.2 Example analysis

We present an example analysis on a data set of fisher movement that is automatically imported with the package amt. Two possible workflows are contrasted: using `amt::random_steps()` and using `add_random()`.

#### C.2.1 Workflow using amt

We first load all required packages, and the fisher data set used in the analysis. We subset the data set to one individual fisher, because the code does not support multiple individuals. (This could be implemented as an extension, but we chose not to for simplicity.)

```
library(miniSSF)
library(amt) # for amt_fisher data set and data prep
library(terra) # for extract() and unwrap()
library(CircStats) # for von Mises distribution

# Load fisher data set from amt
track <- subset(amt_fisher, name == "Lupe")
```

The package amt is available on CRAN, and several vignettes describe the key analysis steps. Here, we only use the package to generate random steps, and this is done as follows:

1. `make_track()` and `steps()` transform the data frame into the format expected by amt;
2. `random_steps()` generates random locations (here $K = 50$);
3. `extract_covariates()` extracts covariate values at the observed and random locations.

By default, `random_steps()` generates random locations based on a gamma distribution of distances and a von Mises distribution of turning angles, so we use this as the importance function in this analysis. The parameters of those distributions (which we will need later) are stored in the output object.

```
# Transform to x/y/t data structure
df <- make_track(tbl = track, .x = x_, .y = y_, .t = t_)

# Use amt to generate random steps and extract covariates
df$burst_ <- 1
elev <- unwrap(amt_fisher_covar$elevation)
df <- df |> steps() |>
    random_steps(n_control = 50) |>
    extract_covariates(elev)
```

For model fitting, we need to create an R function for the probability density of the importance

distribution. The importance distribution is the spatial distribution implied by gamma-distributed step lengths and von Mises-distributed turning angles. As described in Appendix D, this turns out to be proportional to the product of the gamma and von Mises density functions (`dgamma()` and `dvm()`, respectively) *divided by the step length*. We define this as the function `dsamp()`, which also takes arguments for the parameters of the gamma and von Mises distributions (obtained from the amt output).

```r
# Sampling distribution
dsamp <- function(step, angle, ...) {
    args <- list(...)
    dgamma(step, shape = args$shape, scale = args$scale) / step *
        dvm(angle, mu = 0, kappa = args$kappa)
}
# Sampling distribution parameters from amt
amt_par <- list(shape = attr(df, "sl_")$par$shape,
                scale = attr(df, "sl_")$par$scale,
                kappa = attr(df, "ta_")$par$kappa)
```

We define the model formula, which corresponds to the SSF

$$\exp(\beta_1 \times \text{step length} + \beta_2 \times \cos(\text{turning angle}) + \beta_3 \times \text{elevation}),$$

i.e., step length is modelled with a gamma distribution (with fixed shape parameter), turning angle is modelled with a von Mises distribution, and elevation is included as a linear effect. We need to specify starting values for $(\beta_1, \beta_2, \beta_3)$, which is passed to the optimiser for model fitting.

```r
# Model formula
formula <- ~ sl_ + cos(ta_) + elevation
# Starting values for SSF parameters
par0 <- c(-0.03, 0.3, 0)

# Fit model
mod <- ssf(formula = formula, data = df, par0 = par0, dsamp = dsamp,
          shape = amt_par$shape, scale = amt_par$scale, kappa = amt_par$kappa)
mod$estimate
```

```
[1] -0.03253041  0.29979296  0.03741026
```

The output is the object returned by `nlm()`, and we can extract the estimated parameters.

### C.2.2 Workflow using `add_random()`

Alternatively, the function `add_random()` provided above can be used to generate random locations. Here, we explicitly define a function to generate random (gamma) step lengths and (von Mises)

turning angles. The parameters of the importance distribution are chosen based on the data. In the following chunk, `rsamp()` generates points according to the importance distribution, and `dsamp()` is the probability density function, identical to that used in the amt workflow.

```
# Random number generator
rsamp <- function(n, ...) {
    args <- list(...)
    steps <- rgamma(n, shape = args$shape, scale = args$scale)
    angles <- rvm(n, mean = 0, k = args$kappa)
    return(list(sl_ = steps, ta_ = angles))
}
# Probability density function
dsamp <- function(step, angle, ...) {
    args <- list(...)
    dgamma(step, shape = args$shape, scale = args$scale) / step *
        dvm(angle, mu = 0, kappa = args$kappa)
}
# Importance function parameters
library(moveHMM) # to compute step lengths and turning angles
steps <- prepData(track, coordNames = c("x_", "y_"), type = "UTM")
shape <- mean(steps$step, na.rm = TRUE)^2/sd(steps$step, na.rm = TRUE)^2
scale <- sd(steps$step, na.rm = TRUE)^2/mean(steps$step, na.rm = TRUE)
kappa <- as.numeric(vm.ml(na.omit(steps$angle))[2])
```

We use the `add_random()` function to get 50 random locations for each observed step, passing `rsamp` as an argument. Then, we extract the elevation values for all locations using the function `terra::extract()`.

```
df <- add_random(data = track, n_random = 50, rsamp = rsamp,
                 shape = shape, scale = scale, kappa = kappa)
df$elevation <- extract(unwrap(amt_fisher_covar$elevation),
                        df[, c("x_", "y_")])$elevation
```

Once the data have been prepared, the model specification using an R formula and the model fitting with `ssf()` are identical to the other workflow. The estimated SSF parameters are almost identical to the amt analysis, confirming that the two workflows are equivalent.

```
# Model formula
formula <- ~ sl_ + cos(ta_) + elevation
# Starting parameter values for optimisation
par0 <- c(-0.03, 0.3, 0)
```

```r
# Model fitting
mod <- ssf(formula = formula, data = df, par0 = par0,
           dsamp = dsamp, shape = shape, scale = scale, kappa = kappa)
mod$estimate
```

```
[1] -0.0325439  0.2997634  0.0374974
```

## C.3 Examples of sampling distributions

The functions provided above are written in such a way that users can choose the importance distribution that suits their needs. Here, we provide code for the density functions (`dsamp`) and random number generators (`rsamp`) for a number of common importance distributions.

### C.3.1 Uniform on a disc

This corresponds to the "uniform Monte Carlo sampling" design described in the manuscript. Points are generated by simulating step lengths as square roots of uniform samples; this transformation is required to ensure that points are uniformly distributed in space. The density function is constant and, because multiplicative constants do not affect inference, we arbitrarily set it to 1 here.

```r
# Random number generator
rsamp <- function(n, ...) {
    args <- list(...)
    steps <- sqrt(runif(n, min = 0, max = args$max^2))
    angles <- runif(n, min = -pi, max = pi)
    return(list(step = steps, angle = angles))
}

# Probability density function
dsamp <- function(step, angle, ...) {
    args <- list(...)
    rep(1, length(step))
}
```

### C.3.2 Gamma step lengths

If the importance function is the two-dimensional spatial distribution implied by a gamma distribution of step lengths, `dsamp` is the probability density function of the gamma distribution divided by the step length.

```r
# Random number generator
rsamp <- function(n, ...) {
    args <- list(...)
```

```
    steps <- rgamma(n, shape = args$shape, scale = args$scale)
    angles <- runif(n, min = -pi, max = pi)
    return(list(step = steps, angle = angles))
}

# Probability density function
dsamp <- function(step, angle, ...) {
    args <- list(...)
    dgamma(step, shape = args$shape, scale = args$scale) / step
}
```

### C.3.3 Gamma step lengths and von Mises turning angles

If the importance function is the two-dimensional spatial distribution implied by a gamma distribution of step lengths and a von Mises distribution of turning angle, `dsamp` is the product of the gamma and von Mises density functions divided by the step length.

```
# Random number generator
rsamp <- function(n, ...) {
    args <- list(...)
    steps <- rgamma(n, shape = args$shape, scale = args$scale)
    angles <- CircStats::rvm(n, mean = 0, k = args$conc)
    return(list(step = steps, angle = angles))
}

# Probability density function
dsamp <- function(step, angle, ...) {
    args <- list(...)
    dgamma(step, shape = args$shape, scale = args$scale) / step *
        CircStats::dvm(angle, mu = 0, kappa = args$conc)
}
```

### C.3.4 Bivariate normal

Another natural method to generate more integration points in areas where the SSF takes higher values is to sample from the bivariate normal distribution centred on the previous location. The implied distribution of step lengths is the Rayleigh distribution, implemented in the package VGAM, which we use to define `rsamp` and `dsamp`.

```
# Random number generator
rsamp <- function(n, ...) {
    args <- list(...)
```

```r
    steps <- VGAM::rrayleigh(n, scale = args$sigma)
    angles <- runif(n, min = -pi, max = pi)
    return(list(step = steps, angle = angles))
}

# Probability density function
dsamp <- function(step, angle, ...) {
    args <- list(...)
    VGAM::drayleigh(step, scale = args$sigma) / step
}
```

### C.3.5 Regular grid on a disc

The last design that we consider is the uniform quadrature described in the manuscript, which consists of generating points over a regular spatial grid over a disc centred on the previous location. This could be done in several ways. Here, we create a grid over a square, and then only keep the points of this grid that lie inside the inscribed circle. We use a heuristic rule to determine what the resolution of the grid needs to be to obtain the required number of integration points. However, note that this will generally not yield the exact number of points due to the geometric constraints of this procedure.

```r
# Points on a grid
make_grid <- function(R, res) {
    # Create grid on square of side 2R
    x <- seq(0, R, by = res)
    x <- c(- x[length(x):1], x[-1])
    y <- x
    xy <- expand.grid(x, y)

    # Only keep points inside disc of radius R
    d <- sqrt(xy[,1]^2 + xy[,2]^2)
    keep <- which(d <= R)
    grid <- xy[keep,]
    return(grid)
}

# Random number generator
rsamp2 <- function(n, ...) {
    args <- list(...)
    grid <- make_grid(R = args$max, res = sqrt(pi) * args$max/sqrt(n))
```

```r
    steps <- sqrt(grid[,1]^2 + grid[,2]^2)
    angles <- atan2(grid[,2], grid[,1])
    return(list(step = steps, angle = angles))
}

# Probability density function
dsamp2 <- function(x, ...) {
    rep(1, length(x))
}
```

# D Implementation of different movement distributions

Consider a SSF model where both the habitat selection function $w$ and the movement kernel $\phi$ are specified in exponential form. Specifically, assume that we have $\phi(\boldsymbol{x}_{t+1} \mid \boldsymbol{x}_{1:t}) = \exp\{m(\boldsymbol{x}_{1:t}, \boldsymbol{x}_{t+1})\boldsymbol{\beta}_m^\intercal\}$, where $m(\boldsymbol{x}_{1:t}, \boldsymbol{x}_{t+1})$ is a vector of movement variables, and $\boldsymbol{\beta}_m$ a vector of movement parameters. Avgar et al. (2016) explained how different distributions of step lengths (from the exponential family) can be modelled in a step selection function by including the right movement variables in the SSF formula. For example, they suggested that including the step length is equivalent to using an exponential distribution, and including step length and its logarithm corresponds to a gamma distribution. In this appendix, we explain why some care is needed to ensure that the step lengths are modelled with the desired distribution. We do not explicitly include the habitat selection function $w$ in what follows, but the exact same reasoning could be applied if we did.

## D.1 Example: including step length as a covariate

### D.1.1 Model formulation

We start from the simplest example: a step selection function which includes step length as the only covariate. That is, movement is modelled through

$$p(y \mid x) = \frac{\exp(\beta r_{xy})}{\int \exp(\beta r_{xz}) dz},$$

where $r_{xy}$ is the distance from $x$ to $y$ (i.e., the step length). We further assume that $\beta < 0$, i.e., long steps tend to be avoided. This defines a random walk model, where the speed of movement is related to the inverse of $\beta$.

Our focus is to figure out what the distribution of step lengths is under this random walk. Avgar et al. (2016) suggested that they will follow an exponential distribution with rate parameter $-\beta$, but this is actually not the case. To see this, let's first use a simulation.

### D.1.2 Simulations

We simulated a track of length $n = 5000$ from the model above, using the following procedure. We started from $x_1 = (0, 0)$ and then, for $i = 2, 3, \ldots, n$,

1. Generate a large number of proposed points uniformly on a disc centred on $x_{i-1}$, $\{z_1, z_2, \ldots, z_K\}$.
2. For each proposed point $z_k$, calculate the weight $w = \exp(\beta\ r_{xz})$.
3. Select $x_i$ from the proposed points, where each $z_k$ has probability $w_k / \sum_{k=1}^{K} w_k$ to be chosen. (These probabilities approximate the true model shown above, which has an integral in the denominator.)

We implemented this with the selection parameter $\beta = -1$, and with $K = 10^4$ proposed points at each iteration. The radius $R$ of the disc in step 1 needs to be high enough so that steps longer than $R$ would be virtually impossible based on the step selection model; here, its value was chosen as a large quantile of the exponential distribution.

This simulation algorithm can be implemented as shown below.

```
# Selection against step length
beta <- -1
# Radius of disc for simulation
R <- qexp(p = 0.999, rate = -beta)
# Number of random points at each step
npts <- 1e4

# Loop over steps
n <- 5000
xy <- matrix(0, nrow = n, ncol = 2)
for(i in 2:n) {
    # Generate uniform points on disc
    r <- sqrt(runif(npts, 0, R^2))
    b <- runif(npts, -pi, pi)
    pts <- matrix(rep(xy[i-1,], each = npts), ncol = 2) +
        r * cbind(cos(b), sin(b))

    # Evaluate SSF weights (just based on step length here)
    w <- exp(beta * r)

    # Pick next point
    choice <- sample(1:npts, size = 1, prob = w/sum(w))
    xy[i,] <- pts[choice,]
}

head(xy)
```

```
          [,1]      [,2]
[1,]  0.000000  0.000000
[2,]  1.548453 -0.795244
[3,]  2.374106 -1.690673
[4,] -2.048333  1.957159
[5,] -3.932625  2.291976
[6,] -1.936001  6.149087
```

We now have a matrix with two columns, where each row is the coordinates of a point in the track. From this, the step lengths can be calculated as the Euclidean distances between successive points. If we plot of histogram of those step lengths, we can see that their distribution is not an exponential distribution; indeed, its mode is not zero (which is always the case for exponential distributions).

```
# Compare distribution of step lengths to exponential distribution
steps <- sqrt(rowSums((xy[-1,] - xy[-n,])^2))
hist(steps, probability = TRUE, breaks = 50,
     border = "white", ylim = c(0, 1), main = NULL)
grid <- seq(min(steps), max(steps), length = 100)
col <- c("firebrick", "royalblue")
lines(grid, dexp(grid, rate = -beta), lwd = 2, col = col[1])
lines(grid, grid * dexp(grid, rate = -beta), lwd = 2, col = col[2])
legend("top", legend = c("dexp(step)", "step*dexp(step)"),
       col = col, lwd = 2, bty = "n")
```

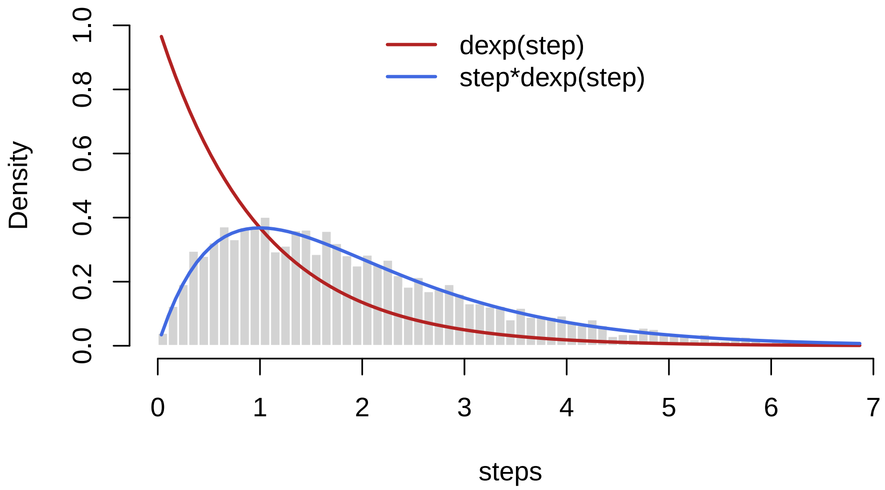


In fact, it turns out that the distribution of step lengths has probability density function proportional to

$$f_r(r) \propto re^{\beta r},$$

which defines a gamma distribution with shape parameter 2 and with rate parameter $-\beta$.

To understand this, we can look at the proposed points for one step, coloured by their weights (which are proportional to their probability of being chosen as the next point in the track). The proposed points that are close to the start point have higher probability, as expected from the formula $\exp(-r_{xz})$. However, a key observation is that there are more proposed points that are at large distances from the start point; e.g., there are more points between 1 and 2 units away from the origin than between 0 and 1 units. This is because the area of a ring centred on the start point increases with the radius of that ring. For this reason, more long steps will be selected than would be expected under an exponential distribution of step lengths.

```r
# Visualise weights for one step
# Weights are much higher in the middle, but many more points on the outside!
library(ggplot2)
theme_set(theme_bw())
df <- data.frame(x = pts[,1], y = pts[,2], w = w)
ggplot(df, aes(x, y, col = w)) +
    geom_point(size = 0.2) +
    coord_equal() +
    scale_color_gradientn(colours = c("grey", "red"))
```

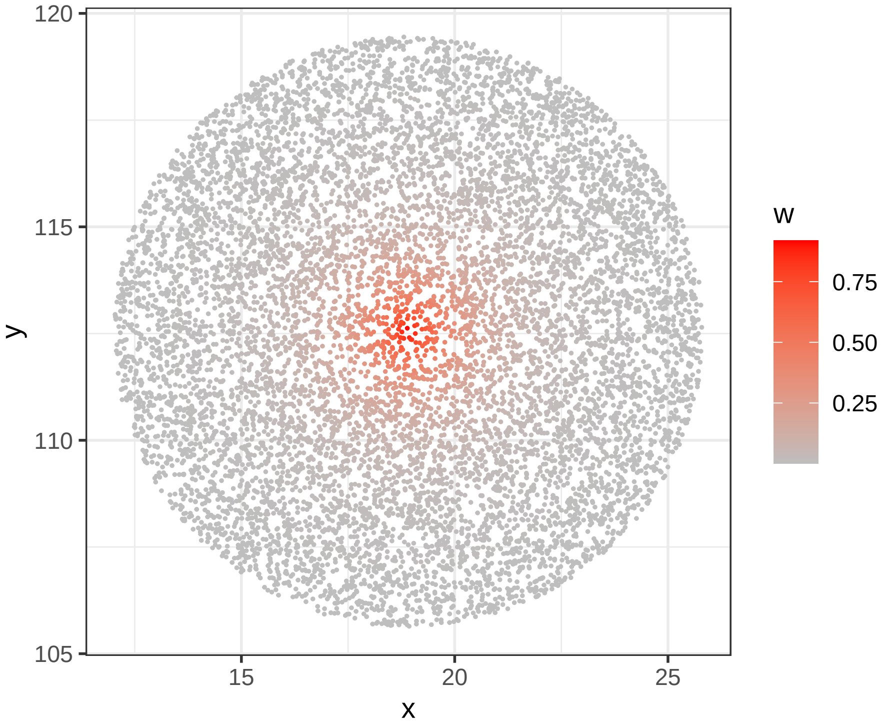


## D.2 Mathematical justification

There are at least two equivalent mathematical approaches in the literature to explain the phenomenon described above. The key result is the relationship between the one-dimensional distribution of step length $f_r$ and the two-dimensional spatial distribution of endpoints $f_{x,y}$.

### D.2.1 Method 1: transformation from polar to Cartesian coordinates

Given the start point of a step, we are interested in the distribution of the next point that the animal selects. We can think of two different ways that this step can be written mathematically:

1. in terms of a change $x$ in Easting and a change $y$ in Northing;

2. in terms of a step length $r$ and bearing $\alpha$.

The probability distribution of interest is different in the two approaches: two-dimensional spatial distribution in the former, and distributions of step length and bearing in the latter. Schlägel and Lewis (2016) (Appendix 2) used a change of variable technique to derive the relationship between the probability density functions that arise from the two approaches.

The relationship between $(x, y)$ and $(r, \alpha)$ is the following:

$$\begin{cases} x = r\cos(\alpha) =: v_1(r, \alpha) \\ y = r\sin(\alpha) =: v_2(r, \alpha) \end{cases}$$

The Jacobian matrix of the transformation is

$$\begin{aligned} J &= \begin{pmatrix} \frac{\partial v_1}{\partial r}(r, \alpha) & \frac{\partial v_1}{\partial \alpha}(r, \alpha) \\ \frac{\partial v_2}{\partial r}(r, \alpha) & \frac{\partial v_2}{\partial \alpha}(r, \alpha) \end{pmatrix} \\ &= \begin{pmatrix} \cos(\alpha) & -r\sin(\alpha) \\ \sin(\alpha) & r\cos(\alpha) \end{pmatrix} \end{aligned}$$

and its determinant is

$$|J| = r\cos(\alpha)^2 + r\sin(\alpha)^2 = r$$

Finally, we can plug this into the general formula for obtaining the probability density function after a change of variable:

$$f_{r,\alpha}(r, \alpha) = |J| f_{x,y}(x, y) = r f_{x,y}(x, y),$$

or, conversely,

$$f_{x,y}(x, y) = \frac{1}{r} f_{r,\alpha}(r, \alpha).$$

The additional factor $r$ in the expression for $f_{r,\alpha}$ above is the factor which shows up in the distribution of simulated step lengths in the above example.

### D.2.2 Method 2: infinitesimal ring

Rhodes et al. (2005) (Appendix B) presented another way to think about this change of variable, leading to the same result. They used a geometrical argument based on the area of a ring of infinitesimal width $dr$ centred on the start point of the step. This area increases proportionally with the radius of the ring, and so the probability is spread over a larger area. This leads to the relationship

$$f_{x,y}(x, y) = \frac{1}{2\pi r} f_r(r).$$

This is equivalent to the formula found from a change of variable, when the bearing is assumed to be uniformly distributed over $(-\pi, \pi]$. Indeed, in that case,

$$f_{r,\alpha}(r, \alpha) = f_r(r) f_\alpha(\alpha) = \frac{1}{2\pi} f_r(r).$$

### D.3 From $f_r$ to $f_{x,y}$

To determine the SSF formulation required for a given distribution of step lengths, $f_r$, we must first transform it into the two-dimensional spatial distribution of endpoints $f_{x,y}$ implied by that distribution, and then write it in the form of an SSF (i.e., exponential form).

#### D.3.1 Exponential distribution

The pdf of the exponential distribution with rate parameter $\lambda$ is $f_r(r) = \lambda e^{-\lambda r}$, so the corresponding spatial distribution is

$$\begin{aligned} f_{x,y}(x, y) &= \frac{1}{2\pi r}\lambda e^{-\lambda r} \\ &= \exp\left[-\lambda r - \log(r)\right] \times \frac{\lambda}{2\pi} \\ &\propto \exp\left[-\lambda r - \log(r)\right], \end{aligned}$$

where we omit the multiplicative term that does not depend on step length $r$.

To model step length with an exponential distribution, we must therefore include step length as a covariate, and an offset for log step length. The coefficient for step length is minus the rate of the distribution.

#### D.3.2 Gamma distribution

The pdf of the gamma distribution with shape parameter $\theta_1$ and rate parameter $\theta_2$ is $f(r) = r^{\theta_1 - 1} e^{-\theta_2 r} \theta_2^{\theta_1} / \Gamma(\theta_1)$, where $\Gamma$ is the gamma function, so the two-dimensional distribution is

$$\begin{aligned} f_{x,y}(x, y) &= \frac{1}{2\pi r} \frac{r^{\theta_1 - 1} e^{-\theta_2 r} \theta_2^{\theta_1}}{\Gamma(\theta_1)} \\ &= \exp\left[-\theta_2 r + (\theta_1 - 1)\log(r) - \log(r)\right] \times \frac{\theta_2^{\theta_1}}{2\pi\Gamma(\theta_1)} \\ &\propto \exp\left[-\theta_2 r + (\theta_1 - 2)\log(r)\right]. \end{aligned}$$

This model requires including step length and log step length as covariates. The selection coefficients are related to the shape and rate through:

$$\begin{cases} \beta_r = -\theta_2 \\ \beta_{\log(r)} = \theta_1 - 2 \end{cases}$$

### D.3.3 Log-normal distribution

The two-dimensional pdf implied by a log-normal distribution of step lengths with location parameter $\mu$ and scale parameter $\sigma$ is

$$\begin{aligned}
f_{x,y}(x,y) &= \frac{1}{2\pi r} \times \frac{1}{r\sigma\sqrt{2\pi}} \exp\left[-\frac{(\log(r)-\mu)}{2\sigma^2}\right] \\
&= \frac{1}{2\pi\sqrt{2\pi}\sigma r^2} \exp\left[-\frac{\log(r)^2 - 2\mu\log(r) + \mu^2}{2\sigma^2}\right] \\
&= \exp\left[-2\log(r) - \frac{1}{2\sigma^2}\log(r)^2 - \frac{\mu}{\sigma^2}\log(r)\right] \times \frac{\exp(-\mu^2/(2\sigma^2))}{2\pi\sqrt{2\pi}\sigma} \\
&\propto \exp\left[-\left(\frac{\mu}{\sigma^2}+2\right)\log(r) - \frac{1}{2\sigma^2}\log(r)^2\right]
\end{aligned}$$

This model requires including log step length and squared log step length as covariates, and the selection coefficients are linked to the distribution parameters through

$$\begin{cases}
\beta_{\log(r)} = -\mu/\sigma^2 - 2 \\
\beta_{\log(r)^2} = -1/(2\sigma^2)
\end{cases}$$

## D.4 From $f_{x,y}$ to $f_r$

Conversely, we can start from a two-dimensional distribution, and derive the implied distribution of step lengths.

### D.4.1 Bivariate normal distribution

Say we want to model the animal's movement as a Gaussian random walk, i.e., each step is an increment from a bivariate normal distribution. A symmetric bivariate normal distribution with mean $(0,0)$ and standard deviation $\sigma$ has pdf

$$f_{x,y}(x,y) = \frac{1}{2\pi\sigma^2} \exp\left[-\frac{r^2}{2\sigma^2}\right]$$

where $r = \sqrt{x^2+y^2}$ is the distance from $(x,y)$ to the mean $(0,0)$. In an SSF, this model could be implemented by including the squared step length as a covariate, and the corresponding selection coefficient would be related to the variance of the normal distribution through $\beta_{r^2} = -1/(2\sigma^2)$.

From this, we derive the distribution of step lengths

$$\begin{aligned}
f_r(r) &= 2\pi r f_{x,y}(x,y) \\
&= \frac{2\pi r}{2\pi\sigma^2} \exp\left[-\frac{r^2}{2\sigma^2}\right] \\
&= \frac{r}{\sigma^2} \exp\left[-\frac{r^2}{2\sigma^2}\right],
\end{aligned}$$

which is the pdf of a distribution known as the Rayleigh distribution.

# References


Avgar, Tal, Jonathan R Potts, Mark A Lewis, and Mark S Boyce. 2016. "Integrated Step Selection Analysis: Bridging the Gap Between Resource Selection and Animal Movement." *Methods in Ecology and Evolution* 7 (5): 619–30.

Klappstein, Natasha Jean, Len Thomas, and Theo Michelot. 2023. "Flexible Hidden Markov Models for Behaviour-Dependent Habitat Selection." *Movement Ecology* 11 (1): 30.

Rhodes, Jonathan R, Clive A McAlpine, Daniel Lunney, and Hugh P Possingham. 2005. "A Spatially Explicit Habitat Selection Model Incorporating Home Range Behavior." *Ecology* 86 (5): 1199–1205.

Schlägel, Ulrike E, and Mark A Lewis. 2016. "A Framework for Analyzing the Robustness of Movement Models to Variable Step Discretization." *Journal of Mathematical Biology* 73: 815–45.
